# Supplementary material for: Modelling heterogeneity in the classification process in multi-species distribution models can improve predictive performance
Source: arXiv:2305.01989 source file (2023-05-03)
Supplement: Supplementary file 1 [file Supplementary.tex]

%\section{Supplementary Information Two for 'Accounting for Misclassification in Multispecies distribution models'.}
\section{Supplementary information 3}

\textbf{Study scenarios and their respective linear predictors for the classification process}.
We present the linear predictors for the study scenarios described in section (2.2) of the classification process in equation (3) of the main paper for the CCM, CSIM and CSICM. 

\subsection*{a) Classification covariate model (CCM)}
The CCM fits the MMGLM defined by equation (4) in the main paper for the classification process. 

\subsection*{b) Classification simplified covariate model (CSIM)}
The CCM fits the MMGLM defined by equation (4) in the main paper by assuming that the covariate that affects the classification process only affects the probability of correctly classifying the state. The linear predictor with covariate $\textbf{z}_{n}$ in equation (4) becomes:
\begin{equation}\label{CSIM}
\begin{split}
\mathbf{\zeta} &=
\mathbf{\omega_0} +  \ldots +\mathbf{\omega_n}*\textbf{z}_{n}\\
&= 
 \begin{bmatrix}
{\omega_0}_{11} & {\omega_0}_{12}&  \cdots& {\omega_0}_{1K}   \\
{\omega_0}_{21} & {\omega_0}_{22}&  \cdots& {\omega_0}_{2K} \\
\vdots & \vdots & \cdots& \vdots\\
{\omega_0}_{S1} & {\omega_0}_{S2} & \cdots& {\omega_0}_{SK} \\
\end{bmatrix}   + \ldots + \begin{bmatrix}
{\omega_n}_{\cdot} & 0 &  \cdots&0 &  \cdots& 0   \\
0 & {\omega_n}_{\cdot}& \cdots& 0 &  \cdots& 0 \\
\vdots & \vdots &  \cdots& \vdots\\
0 & 0 &  \cdots&{\omega_n}_{\cdot} &  \cdots&0 \\
\end{bmatrix}* \textbf{z}_{n},
\end{split}
\end{equation}
where ${\omega_n}_{\cdot}$ are assumed to be the same for all the verified states. Since the rows of $\mathbf{\Omega}$ sum to 1, the heterogeneity is introduced through the variation in the probability of correctly classifying the verified states. 

\subsection*{c) Classification simplified intercept covariate model (CSICM)}
We can further reduce the number of parameters estimated in equation \eqref{CSIM} by also assuming that the intercept for correctly classifying the state are the same. In this case, the linear predictor of the classification process becomes:

\begin{equation}\label{CSIM}
\begin{split}
\mathbf{\zeta} &=
\mathbf{\omega_0} +  \ldots +\mathbf{\omega_n}*\textbf{z}_{n}\\
&= 
 \begin{bmatrix}
{\omega_0}_{\cdot} & {\omega_0}_{12}&  \cdots& {\omega_0}_{1k}&\cdots & {\omega_0}_{1K}   \\
{\omega_0}_{21} & {\omega_0}_{\cdot}&  \cdots& {\omega_0}_{2k}&\cdots & {\omega_0}_{2K} \\
\vdots & \vdots & \cdots& \vdots\\
{\omega_0}_{S1} & {\omega_0}_{S2} & \cdots& {\omega_0}_{\cdot}&\cdots & {\omega_0}_{SK} \\
\end{bmatrix}   + \ldots + \begin{bmatrix}
{\omega_n}_{\cdot} & 0 &  \cdots&0 &  \cdots& 0   \\
0 & {\omega_n}_{\cdot}& \cdots& 0 &  \cdots& 0 \\
\vdots & \vdots &  \cdots& \vdots\\
0 & 0 &  \cdots&{\omega_n}_{\cdot} &  \cdots&0 \\
\end{bmatrix}* \textbf{z}_{n},
\end{split}
\end{equation}
where ${\omega_n}_{\cdot}$ are assumed to be the same for all the verified states. Since the rows of $\mathbf{\Omega}$ sum to 1, the heterogeneity is introduced through the variation in the probability of correctly classifying the verified states.
