# Supplementary material for: Modelling heterogeneity in the classification process in multi-species distribution models can improve predictive performance
Source: arXiv:2305.01989 source file (2023-05-03)
Supplement: Supplementary file 2 [file Supplementary1.tex]

%\section{Supplementary Information Two for 'Accounting for Misclassification in Multispecies distribution models'.}
\section{Supplementary information 1}

\textbf{Equivalent Representation of Equation (1) and (2) to the multinomial logit model}.

We want to show that the model definition for the verified species in the main text can be easily modified to the multinomial logit model. Given the data with $c= 1,2,\ldots, C+1$ categories, \cite{Fahrmeir2013} defined the multinomial logit model as described below

\begin{equation} \label{multinomial logit}
    log(\frac{\pi_c}{\pi_{C+1}}) = X'\beta,
\end{equation}
where $\pi_c$ is the probability of observing category $c$, $\pi_{C+1}$ is the probability of observing reference category $C+1$, $\beta$ is a vector of coefficients and $X$ is the design matrix.

Let us define $s'$ as the reference species, for $s' \in \{1,2,\ldots, S\}$. Given the intensity for the species $s$ as defined by equation (1), then the proportion of having verified species $s$ as defined by equation (2) becomes:

\begin{equation}
    \begin{split}
        p_{is} = P(\text{verified species} = s)= \frac{e^{\beta_{0s} + \beta_{1s} x_i}}{\sum_s e^{\beta_{0s} + \beta_{1s} x_i}}
    \end{split}
\end{equation}

The ratio of the proportion of observing verified species $s$ relative to the reference verified species $s'$ at site $i$ becomes:
\begin{equation}
    \begin{split}
        \frac{p_{is}}{p_{is'}} &= \frac{e^{\beta_{0s} + \beta_{1s} x_i}}{e^{\beta_{0s'} + \beta_{1s'} x_i}}\\
        \implies log \bigg(\frac{p_{is}}{p_{is'}} \bigg) &= (\beta_{0s} - \beta_{0s'}) + (\beta_{1s} - \beta_{1s'})x_i\\
        &= X'\beta
    \end{split}
    \label{mylogit}
\end{equation}
which is the same as the multinomial logit model defined in equation \eqref{multinomial logit}.
