# Supplementary material for: Modelling heterogeneity in the classification process in multi-species distribution models can improve predictive performance
Source: arXiv:2305.01989 source file (2023-05-03)
Supplement: Supplementary file 3 [file Supplementary2.tex]

\section{Supplementary Information 2}
\subsection*{Model Representation as a general form of misclassification in multispecies SDMs.}

Our proposed model in the main text is a generalisation of the model framework proposed by \cite{wright2020modelling} which provides a general framework for modelling misclassification in multispecies distribution models. We first present our model into the model framework described by \cite{wright2020modelling} and then by the deductions made in their paper, establish the generalisations of our framework. Since \cite{spiers2022estimating} is an extension of the work by \citep{wright2020modelling}, their work fits into our model framework.

\subsection*{a. Model Framework by \cite{wright2020modelling}.}

Let $z_j$ be the true presence/absence state for site $j$. Then $z_j \sim \text{Bernoulli}(\psi_j)$, where $\psi_j$ is the occupancy probability. Let $Y_{ij}$ be the latent detection counts for each species $i$ at site $j$, that is, $Y_{ij} \sim \text{Poisson} (\lambda_i)$ and the observed counts given the latent detection counts $[C|Y=y] \sim \text{Multinomial}(y, \Theta)$, where C and $\Theta$ are K-length vectors and $\Theta$ is the confusion matrix.

The joint distribution of C and Y is then:
\begin{equation*}
    \begin{split}
        P(C=c,Y=y) &= Pr(C=c|y=y) P(Y=y)\\
        &= \bigg[\frac{1}{c_1!} (\lambda \theta_1)^{c_1}e^{-\lambda \theta_1}\bigg] \bigg[\frac{1}{c_2!} (\lambda \theta_2)^{c_2}e^{-\lambda \theta_2}\bigg] \cdots \bigg[\frac{1}{c_k!} (\lambda \theta_k)^{c_k}e^{-\lambda \theta_k}\bigg]
    \end{split}
\end{equation*}
and as such the probability mass function for each $c_k$ is that of a Poisson distribution with rate parameter $\lambda \theta_k$. Hence $[C_{ik.k'}|Z_i] \sim \text{Poisson} (\sum_{k=1}^K z_{ik} \lambda_{ij} \theta_{kk'})$, where $z_i$ is the vector of occupancy at site $i$ for all $K$ species used in their studies.

\subsection*{b) Connection between our framework and that of \cite{wright2020modelling}.}
The deductions made by \cite{wright2020modelling} hangs on the proof that the marginal distribution of the observed species counts being Poisson. We therefore show that the distribution of the observed counts (reported category) are Poisson distributed, and as well all the deductions by \citep{wright2020modelling} holds. 

The hierarchical likelihood of the model in the main article was:
\begin{equation*}
    \begin{split}
        \ln (\lambda_{is}) &= \textbf{x}'\beta \\
        p_{is} &= \frac{\lambda_{is}}{\sum_i \lambda_{is}}\\
                Y_{i} &\sim Poisson (\Lambda = \sum_{s=1}^S \lambda_{is}) \\
        V_{i} | Y_{i} & \sim Categorical(p_{i.})\\
        \textbf{C}_i | {V}_{i}& \sim categorical(\Omega_{V_i, \cdot})
    \end{split}
\end{equation*}
where $\textbf{C}$ denotes the reported or observed category, $\textbf{V}$ denotes the verified state and ${Y}$ denotes the total number of verified states for site $i$ for $s= 1, \ldots, S$ verified states, $k=1,2,\ldots, K$ reported categories and $i=1, 2, \ldots,R$ number of sites. It must be noted that the categorical distribution used in the main article is the multinomial distribution with $Y=1$ for all the sites, since we assumed that we can only observe one state at a site. In that case, 

\begin{equation}
    P(Y=1) = \Lambda e^{-\Lambda}
\end{equation}

The joint distribution of $\textbf{V}$ and $Y$ is:
\begin{equation}
\begin{split}
    P(\textbf{V}=\textbf{v}, Y=1) &= \bigg[ \  p_1 ^{v_1}p_2 ^{v_2} \cdots p_s ^{v_s}\bigg] \bigg[ \Lambda^y e^{-\Lambda}\bigg] \\
    &= \bigg[ (\Lambda p_{1})^{v_1} e^{-\Lambda p_{1}}\bigg]\bigg[  (\Lambda p_{2})^{v_2} e^{-\Lambda p_{2}}\bigg] \cdots\bigg[(\Lambda p_{s})^{v_s} e^{-\Lambda p_{s}}\bigg] 
    \end{split}
\end{equation}
This implies that the marginal distribution of each verified state $V_s$ is a Poisson distribution with rate parameter $\Lambda p_s$. 

We then proceed to find the marginal distribution of the reported counts $C_k$ for each category given the verified state $v_s$,:
\begin{equation}
    \begin{split}
   P(\textbf{C}=\textbf{c}, V_s= 1) &= P(\textbf{C}=\textbf{c}| V_s= 1)P(V_s= 1)\\
   &= \Omega_{s1}^{c_1}\Omega_{s2}^{c_2} \cdots \Omega_{sK}^{c_K} (\Lambda p_s)e^{\Lambda p_s}\\
   &=\prod_k (\Lambda p_s \Omega_{sk})^{c_k}e^{-\Lambda p_s\Omega_{sk}}
    \end{split}
\end{equation}
where $\Omega_{sk}$ is the sth row and kth column of the confusion matrix $\Omega$ in equation (3) of the main paper. This equation shows that the marginal distribution of the observed or reported counts $C_k$ are Poisson distributed with rate parameter $\Lambda p_s\Omega_{sk}$.

Our result is similar to that of \cite{wright2020modelling}, with the rate parameter of our proposed model scaled by the probability of the verified state $p_s$.

\subsection*{c) Extensions to the other models.}

With the discussions above, we can state that our model is also a generalisation of the two species with binary detection \citep{chambert2018two}, single species with count detections \citep{chambert2015modeling} and single species with binary detections \citep{chambert2018new} with the proof explained by \cite{wright2020modelling}. It can also be extended for other non-occupancy models as explained by \cite{wright2020modelling}.
