# Supplementary material for: Modelling heterogeneity in the classification process in multi-species distribution models can improve predictive performance
Source: arXiv:2305.01989 source file (2023-05-03)
Supplement: Supplementary file 4 [file Supplementary_information1.tex]

\section{Supplementary Information One (S1) for 'Modelling heterogeneity in classification process in multi-species distribution models improves predictive performance.'}

\textbf{Equivalent Representation of Equation (1) and (2)}.

We want to show that the model definition for the verified species in the main text is the multinomial logit model. Given the data with $c= 1,2,\ldots, C+1$ categories, \cite{Fahrmeir2013} defined the multinomial logit model as described below

\begin{equation} \label{multinomial logit}
    log(\frac{\pi_c}{\pi_{C+1}}) = X'\beta,
\end{equation}
where $\pi_c$ is the probability of observing category $c$, $\pi_{C+1}$ is the probability of observing reference category $C+1$, $\beta$ is a vector of coefficients and $X$ is the design matrix.

Let us define $i'$ as the reference species, for $i' \in \{1,2,\ldots, S\}$. Given the intensity for the species $i$ as defined by equation \eqref{intensity}, then the proportion of having verified species $i$ as defined by equation \eqref{proportion} becomes:

\begin{equation}
    \begin{split}
        p_{ij} = P(\text{verified species} = i)= \frac{e^{\beta_{0i} + \beta_{1i} x_j}}{\sum_i e^{\beta_{0i} + \beta_{1i} x_j}}
    \end{split}
\end{equation}

The ratio of the proportion of observing verified species $i$ relative to the reference verified species $i'$ at site $j$ becomes:
\begin{equation}
    \begin{split}
        \frac{p_{ij}}{p_{i'j}} &= \frac{e^{\beta_{0i} + \beta_{1i} x_j}}{e^{\beta_{0i'} + \beta_{1i'} x_j}}\\
        \implies log \bigg(\frac{p_{ij}}{p_{i'j}} \bigg) &= (\beta_{0i} - \beta_{0i'}) + (\beta_{1i} - \beta_{1i'})x_j\\
        &= X'\beta
    \end{split}
\end{equation}
which is the same as the multinomial logit model defined in equation \eqref{multinomial logit}.
