# Supplementary material for: Modelling heterogeneity in the classification process in multi-species distribution models can improve predictive performance
Source: arXiv:2305.01989 source file (2023-05-03)
Supplement: Supplementary file 5 [file supplementary3.tex]

\section{supplementary 4}

\begin{sidewaystable}
\setlength\tabcolsep{2pt} % default is '6pt'
\setlength\extrarowheight{2pt}
\caption{Trabalhos Selecionados após critérios de Seleção} 
\label{tab:laal} 
\begin{tabularx}{\textwidth}{|*{16}{C|}}
\hline
Identificador &
Autores & 
Ano & 
Titulo &
Resumo & 
Benefícios & 
Limitações & 
Padrão de Projeto & 
Elementos\slash Padrões Arquiteturais & 
Tecnologias (frame\-works, APIs) & 
Modelo de Acessibilidade & 
Nível Acessibilidade & 
Tipo de Deficiência & 
Tecnologia Assistiva & 
Linguagens & 
Tipo de Avaliação \\ 
\hline
\end{tabularx}

\end{sidewaystable}

\begin{table}[ht!]
\tablestyle[sansbold]
\begin{tabular}{*{8}{p{0.1\textwidth}}}
\theadstart
        experience & "truth" & Queen & Monarch & Viceroy & other & other danaus & other limenitis \\ 
        \tbody
        
        \hline
        1 & Queen & 4442 & 0 & 0 & 0 & 0 & 0 \\ \hline
        1 & Monarch & 86 & 6780 & 9 & 127 & 1 & 0 \\ \hline
        1 & Viceroy & 2 & 3 & 619 & 2 & 1 & 0 \\ \hline
        2 & Queen & 944 & 0 & 0 & 0 & 0 & 0 \\ \hline
        2 & Monarch & 19 & 1624 & 6 & 18 & 0 & 0 \\ \hline
        2 & Viceroy & 1 & 2 & 201 & 1 & 0 & 2 \\ \hline
        3 & Queen & 687 & 0 & 0 & 0 & 0 & 0 \\ \hline
        3 & Monarch & 10 & 921 & 3 & 30 & 0 & 0 \\ \hline
        3 & Viceroy & 0 & 1 & 90 & 0 & 0 & 1 \\ \hline
        4 & Queen & 110 & 0 & 0 & 0 & 0 & 0 \\ \hline
        4 & Monarch & 3 & 196 & 0 & 79 & 0 & 0 \\ \hline
        4 & Viceroy & 0 & 0 & 13 & 0 & 0 & 0 \\ \hline
        5 & Queen & 18 & 0 & 0 & 0 & 0 & 0 \\ \hline
        5 & Monarch & 3 & 272 & 0 & 3 & 0 & 0 \\ \hline
        6 & Queen & 384 & 0 & 0 & 0 & 0 & 0 \\ \hline
        6 & Monarch & 2 & 600 & 1 & 38 & 0 & 0 \\ \hline
        6 & Viceroy & 0 & 0 & 102 & 0 & 0 & 0 \\ \hline
 \tend
\end{tabular}
    \caption{Crosstabulation of the verified states and reported categories for the training set of the butterfly dataset. The training set was used in fitting the model, and the experience level was used as a covariate in the classification process.}
    \label{training data}
\end{table}

\begin{table}[ht!]
\tablestyle[sansbold]
\begin{tabular}{*{8}{p{0.1\textwidth}}}
\theadstart
        experience & "truth" & Queen & Monarch & Viceroy & other & other danaus & other limenitis \\ 
        \tbody
        
        \hline
      1 & queen & 1792 & 0 & 0 & 0 & 0 & 0 \\ \hline
        1 & Monarch & 12 & 4080 & 1 & 56 & 1 & 0 \\ \hline
        1 & Viceroy & 0 & 3 & 150 & 0 & 0 & 0 \\ \hline
        2 & queen & 192 & 0 & 0 & 0 & 0 & 0 \\ \hline
        2 & Monarch & 3 & 570 & 0 & 3 & 1 & 0 \\ \hline
        2 & Viceroy & 0 & 0 & 16 & 0 & 0 & 0 \\ \hline
        3 & queen & 202 & 0 & 0 & 0 & 0 & 0 \\ \hline
        3 & Monarch & 1 & 430 & 0 & 0 & 0 & 0 \\ \hline
        3 & Viceroy & 0 & 0 & 12 & 0 & 0 & 0 \\ \hline
        4 & queen & 118 & 0 & 0 & 0 & 0 & 0 \\ \hline
        4 & Monarch & 0 & 113 & 0 & 0 & 0 & 0 \\ \hline
        4 & Viceroy & 0 & 0 & 4 & 0 & 0 & 0 \\ \hline
        5 & queen & 5 & 0 & 0 & 0 & 0 & 0 \\ \hline
        5 & Monarch & 0 & 156 & 0 & 0 & 0 & 0 \\ \hline
        6 & queen & 137 & 0 & 0 & 0 & 0 & 0 \\ \hline
        6 & Monarch & 0 & 272 & 0 & 0 & 0 & 0 \\ \hline
        6 & Viceroy & 0 & 0 & 19 & 0 & 0 & 0 \\ \hline
 \tend
\end{tabular}
    \caption{Crosstabulation of the verified states and reported categories for the validation set of the butterfly dataset. The validation set was used in assessing the predictive performance of the model, and the experience level was used as a covariate in the classification process.}
    \label{tab:validation_data}
\end{table}
